# Supplementary material for: Figures as Interfaces: Toward LLM-Native Artifacts for Scientific Discovery
Source: arXiv:2604.08491 source file (2026-10-18)
Supplement: Supplementary file 1 [file 06-appendix.tex]

% \newpage

% \section{Supplementary Note}
% \label{section:appendix}
% % Notion: https://www.notion.so/scisci/Prepare-SI-Design-Space-vis-actions-global-variables-there-are-many-things-predefined-1ce3589a439f8010af5ce109727cf84f?source=copy_link


% \subsection{Action Space} 
% \label{subsection:appendix-action-space}

% \subsubsection{Action Definition}
% Table of actions: name, description, input and output, example (corresponds to the example library) % organic vs. 无机 actions

% claim: we do not claim the completness of this action space. but as an illustration.

% % \begin{figure}[H]
% %     \centering
% %     \includegraphics[width=1\linewidth]{figures/action-space.jpg}
% %     \caption{Action Space}
% %     \label{fig:enter-label}
% % \end{figure}
% % \begin{figure}[H]
% %     \centering
% %     \includegraphics[width=1\linewidth]{figures/action-space-table.jpg}
% %     \caption{Action Space Definition}
% %     \label{fig:enter-label}
% % \end{figure}
% % Final version: https://www.notion.so/scisci/1943589a439f80909770d6bab7add251?v=1943589a439f80b9be08000cf0f09245&source=copy_link 
% % Additional Python Tool definition: https://www.notion.so/scisci/tool-1f83589a439f80c7b422d0297d104886?source=copy_link
% % Original version: https://www.notion.so/scisci/1523589a439f80f78ec6e986855442b8?v=1523589a439f8133a5a9000c28f8cfb1&source=copy_link

% \begin{table}[t]
% \centering
% \caption{
% \newlyadded{Action Definition} 
% }
% \label{tab:example}
% \begin{tabularx}{\linewidth}{llXc}
% \toprule
% Action Type & Action Name & Description & Programming Language \\
% \midrule

% % 假设 Scatter Plot 总共 5 行（3 + 2）
% \multirow{5}{*}{Data Filtering}
%   & \actionname{select_table}
%   & Selects the appropriate tables based on the provided question and table descriptions, and generates a complete SQL query with a SELECT clause and a FROM clause. 
%   & SQL \\
  
%   & \actionname{project_columns}
%   & Based on the provided question, previous SQL query, and table description, automatically select the most relevant columns from the table and generate a new SQL query that replaces SELECT * with a SELECT clause listing only the chosen columns. If the question does not specify any key columns, output the original SQL query unchanged. The output query should be fully qualified for Google BigQuery. 
%   & SQL \\

%   & \actionname{filter_rows}
%   & Filter rows based on question, table description, and previous SQL. 
%   & SQL \\

%   & \actionname{join}
%   & Determine the appropriate join operation and modify the previous SQL query by incorporating a JOIN clause. Use this action when the current SQL query cannot fully answer the user's question, especially when additional information is required. Infer that additional data fields from other tables are needed to complete the query. Based on the provided question and table description, generate a complete SQL query that is fully qualified for Google BigQuery.
%   & SQL \\

%   & \actionname{union}
%   & Combines two SQL queries using the UNION DISTINCT operator if they are union-compatible. Based on the provided question and table description, automatically determine an additional SQL query.
%   & SQL \\
  
% \multirow{6}{*}{Data Transformation}
%   & \actionname{sort}
%   & Modifies the given SQL query by incorporating an ORDER BY clause based on the provided question and table description. The output SQL query should be complete and fully qualified to query Google BigQuery.
%   & SQL \\

%   & \actionname{group_by}
%   & Modifies the given SQL query by incorporating a GROUP BY clause based on the provided question and table description. The output is a complete SQL query suitable for Google BigQuery. 
%   & SQL \\

%   & \actionname{bin}
%   & Based on the provided question and table description, automatically determine whether a numeric column should be binned, choose the appropriate numeric column and a suitable bin width, and modify the previous SQL query by applying a binning operation. The output SQL query should be fully qualified for Google BigQuery.
%   & SQL \\

%   & \actionname{pivot}
%   & Transforms the given SQL query into a pivot query by converting distinct values in a chosen pivot column into separate columns, aggregating a selected value column using a chosen aggregation function, and grouping by appropriate columns. The output is a complete SQL query suitable for Google BigQuery
%   & SQL \\
  
%   & \actionname{sample}
%   & Modifies the given SQL query to return a random sample of rows based on the provided question. Parse the question to determine if a sample size is specified (a probability between 0 and 1). The output query should be fully executable on Google BigQuery.
%   & SQL \\

%   & \actionname{derive_column}
%   & Derives a new column from one or more columns in the given data tables based on the provided user question. Usually will use a mathematical formula (e.g., lambda x: f(x)), string manipulation (e.g., SPLIT(p.journal_name, ' ')[OFFSET(0)], date manipulation (e.g., EXTRACT(MONTH FROM p.publish_date)) to derive the new column. 
%   & SQL \\

% \multirow{4}{*}{Data Analysis}
%   & \actionname{text_embedding}
%   & Based on the provided question and the input DataFrame, automatically choose an appropriate text embedding method (e.g., SciBERT, Sentence-BERT) and generate plain Python code.
%   & Python \\

%   & \actionname{dimension_reduction}
%   & Based on the provided question and DataFrame, choose an appropriate dimension reduction method (PCA, t-SNE) and generate plain Python code. 
%   & Python \\

%   & \actionname{clustering}
%   & Based on the question and the DataFrame, automatically choose an appropriate clustering algorithm among KMeans, DBSCAN, Hierarchical Clustering, or other clustering algorithms, and generate Python code.
%   & Python \\

%   & \actionname{text_summarization}
%   & Based on the provided question and the input DataFrame, generate plain Python code that automatically choose one or more text columns for summarization and summarize the text content by calling the LLM API using the executePrompt() function. 
%   & Python \\

% \multirow{9}{*}{Data Visualization}
%   & \actionname{add_chart_type}
%   & Given a user query and the generated dataframe, (1) choose the most suiteble chart type from given the chart list to answer the user question, and (2) generate a new data visualization dashboard using the vega-lite specification code for this chart type. This tool will return the vega-lite code for the new chart type, with the `mark` field updated. Typically, this is the start of creating a new data visualization dashboard.
%   & Vega-Lite \\

%   & \actionname{add_data}
%   & Add the generated dataframe into the `data` field of a NEW Vega-Lite specification, based on the user query, the generated dataframe, and the existing data visualization vega-lite specification code. This action is only triggered when a chart has just been created and its Vega-Lite spec contains an empty or missing `data` block. The action must FILL IN the previously empty `data` field, without modifying any other parts of the specification. The output is the Vega-Lite specification with the `data` field successfully populated.
%   & Vega-Lite \\

%   & \actionname{add_encoding}
%   & Add one or more NEW visual channels to the `encoding` field of an existing Vega-Lite specification, based on the user query, the generated dataframe, and the existing data visualization vega-lite specification code. This action is invoked ONLY when the user question requires adding additional visual encodings (e.g., color, size, opacity, stroke). The agent must NOT modify or override existing encodings—only append new ones. The chosen visual channels must be semantically meaningful and directly necessary for answering the user's analytical question. Avoid adding redundant or visually unhelpful channels. The output should be the updated Vega-Lite JSON spec with the new encodings inserted in the `encoding` field.
%   & Vega-Lite \\

%   & \actionname{add_params}
%   & Add one or multiple new interaction types (such as click, brush, hover, etc) to the 'params' field to the vega-lite code. It will return the updated vega-lite code with the `param` field updated and the `encoding` field also updated (e.g., add `condition` to the `encoding` field). The interaction types are pre-defined based on the chart type and will not be changed.
%   & Vega-Lite \\

%   & \actionname{add_chart_title_and_caption}
%   & Given a user query, the generated dataframe, and an existing data visualization vega-lite specification code, summarize the data insights and add a title and caption to the vega-lite spec. This tool will return the updated vega-lite code with the `title` and `description` fields updated.
%   & Vega-Lite \\

%   & \actionname{add_chart_config}
%   & Given a user query, the generated dataframe, and an existing data visualization vega-lite specification code, add a chart config to the vega-lite spec. Specifically, this tool can add the chart config into the existing vegalite code. This tool will return the updated vega-lite code with the `config` field updated.
%   & Vega-Lite \\

%   & \actionname{update_data}
%   & Update the `data` field of an EXISTING Vega-Lite specification using the newly generated dataframe, based on the user query, the generated dataframe, and the existing data visualization vega-lite specification code. This action is only invoked when the chart already contains a valid Vega-Lite specification (i.e., the visualization has been previously created and is non-empty). The action must REPLACE the current `data` block without altering any other parts of the specification. The output is the updated Vega-Lite spec with the new dataframe assigned to `data`.
%   & Vega-Lite \\

%   & \actionname{update_encoding}
%   & Modify one or more EXISTING visual channels inside the `encoding` block of a Vega-Lite specification, based on the user query, the generated dataframe, and the existing data visualization vega-lite specification code. This action is invoked only when the chart already has a non-empty `encoding` field, and the user query explicitly requires adjusting the current visual mappings (e.g., changing an existing color channel, altering size mapping, updating axis fields). The agent must NOT add new encodings or remove existing ones--only update the specified channels. All other parts of the Vega-Lite specification must remain unchanged. The output is the updated Vega-Lite JSON specification reflecting the modified encodings.
%   & Vega-Lite \\

%   & \actionname{update_chart_title_and_caption}
%   & Update the chart `title` and `description` fields based on the user's question and the analytical insights derived from the generated dataframe, and the existing data visualization vega-lite specification code. This action updates ONLY the `title` and `description` fields of an existing Vega-Lite specification without modifying any other part of the visualization. The goal is to produce a concise, accurate summary of what the chart shows and how it answers the user's question. The output is the updated Vega-Lite specification with revised title and caption.
%   & Vega-Lite \\

% \multirow{2}{*}{Flag}
%   & \actionname{FINISH_GENERATE}
%   & This action is used to indicate that the task of generating a new chart (i.e., a new vega-lite specification) has been completed. 
%   & -- \\

%   & \actionname{FINISH_UPDATE}
%   & This action is used to indicate that the task of refining and updating the existing chart (i.e., the existing vega-lite specification) has been completed. 
%   & -- \\


% \bottomrule
% \end{tabularx}
% \end{table}


% \subsubsection{Design Space for Visualization Generation}
% \textbf{Visualization Design Space.} 
% 1. Design Space 1: data fact to chart type
% 2. Design Space 2: interaction space
% \wyf{Yifang TODO: update the prompt "the most suitable chart" to Calliope design space (but should be SciSci-oriented)}
% % 3. what else? 
% % data visualization: 
%     % TODO: add design space from task to chart type (add_mark); - add vis task--chat type design space from manually labeled SciSci papers + existing vis paper design space (calliope): to enable a more precise selection of chart types based on user queries/tasks 
%     % add a complete design space about chart interaction; 
% % add vis task--chat type design space from manually labeled SciSci papers + existing vis paper design space (calliope): to enable a more precise selection of chart types based on user queries/tasks



% \subsubsection{Action Dependency Graph}
% \label{subsubsection:appendix-action-dependency-graph}
% We use a two-layer graph to construct the dependency graph among actions, based on the data analysis procedure. 
% % 2-1. How to construct action dependency graph: show the graph visualization, and the code (using action_space.json as input, set precondition and post-condition, to get the dependency graph): code: `/home/yifangwang/visual-gpt/visual-gpt-backend/function/v4/database`
% \begin{figure}[H]
%     \centering
%     \includegraphics[width=1\linewidth]{figures/action_dependency_graph.png}
%     \caption{Action dependency graph}
%     \label{fig:action-dependency-graph}
% \end{figure}




% \subsubsection{Generalizability}
% The action space could be easily adjusted to other science fields beyond SciSci in computational social science and broader data science by human experts or LLM agents. 
% % - action library: could be edited to adjust to other science fields beyond SciSci/CSS — by replaces and extended by human experts or LLM agents (create new agents based on user queries)
% % 1. data filtering/transformation: well-extablished SQL operation
% % 2. data analysis: frequently used models mentioned in SciSci survey paper
% % 3. data visualization: 
%     % TODO: add design space from task to chart type (add_mark); - add vis task--chat type design space from manually labeled SciSci papers + existing vis paper design space (calliope): to enable a more precise selection of chart types based on user queries/tasks 
%     % add a complete design space about chart interaction; 
%     % add mechanisms about linking user's GUI interaction to backend data (how to coordinate -- using vegalite解析 to SQL re-generation, ...) Vis coordination部分 
%     % Coordination: 详细介绍--ID based indexing. 和User management db link在一起
% (4) Justification: Atomic Action Decomposition vs. End-to-End NL2SQL
% % Why Not Use Existing NL2SQL Tools Directly?
% % 1. Scalability & Flexibility Limitations:
% % <cite index="23-1">Current NL2SQL approaches face significant limitations including semantic ambiguity, schema mapping challenges, and difficulties with complex cross-domain queries. Breaking down SQL queries into modularized sub-queries reduces complexity of the original query and mitigates parsing difficulties.</cite>
% % 2. Error Detection & Interpretability:
% % <cite index="25-1">Recent benchmarks reveal that current large language models exhibit significant limitations in semantic error detection for NL2SQL, achieving only 75.16% average detection accuracy. Semantic errors in widely-used datasets like BIRD affect 6.91% of queries.</cite>
% % 3. Action-Level Control Benefits:
% % <cite index="31-1">Task division in NL2SQL can be beneficial, increasing performance by more than 10% compared to direct approaches. Dividing schema linking prompts to capture maximum information about database schema improves performance by a further 10%.</cite>
% % 4. Complex Query Handling:
% % <cite index="28-1">Real-world production data presents challenges including data formatting variations, semantic ambiguity, syntactic rigidity of SQL, and custom business metrics that require more sophisticated decomposition approaches than end-to-end methods can provide.</cite>
% % 5. Multi-Step Query Support:
% % <cite index="27-1,30-1">Advanced NL2SQL systems increasingly require multi-step approaches with safety checks, validation, and context management that are better served by atomic action composition rather than monolithic query generation.</cite>
% % Technical Advantages of Our Approach:

% % Modularity & Reusability: Each atomic action (select\_table, project\_column, filter\_rows, etc.) can be independently optimized and reused across different query patterns.
% % Error Isolation: When failures occur, they can be traced to specific atomic operations, enabling precise debugging and correction.
% % Incremental Complexity: Complex analytical workflows can be built incrementally by composing simpler, verified operations.
% % Transparency: Users can inspect the exact sequence of operations, understanding how their natural language query was interpreted and executed.
% % \textbf{Adaptive Planning: The tree-of-thoughts planning approach can explore multiple decomposition strategies and select optimal action sequences.} % this is very important


% \subsection{Tree-based Planning}
% \label{subsection:si-tree-based-search}
% In the \planner Agent, we use a tree based planning algorithm to help the agent search for candidate actions over the action space (Sec.~\ref{subsection:method-llm}). 
% A sequence of actions from the root to the leaf node represents a complete candidate solution to the user's query. 
% To optimize memory efficiency during search, the tree is constructed using depth-first search (DFS), following three iterative phases: 
% % The tree is constructed using depth-first search (DFS) to optimize memory efficiency through three iterative phases: 
% \begin{itemize}
%     \item \textbf{\textit{Selection}} identifies the optimal candidate action with lowest estimated cost. 
%     \item \textbf{\textit{Expansion}} expands the selected action node by generating subsequent candidate actions, guided by four specialized sub-agents responsible for data filtering, transformation, modeling, and visualization. 
%     \item \textbf{\textit{Update}} revises the costs for newly added nodes, using a score $f(n) = g(n) + h(n)$, where $g(n)$ represents the cumulative execution cost from root to node $n$, and $h(n)$ estimates the future cost to reach the analytical goal.
%     \wyf{TODO: change to tree-of-thought method. do not explictly mention A*. to add the functions for $g(n)$ and $h(n)$}
%     % https://chatgpt.com/share/6944d453-de04-8003-a190-d53f866e9c48
%     % TODO: 让Claude/DeepSeek写出一个优化方程。根据ToolChain那篇文章修改--一开始planner生成一个initial plan，然后根据相似度啥的改
% \end{itemize}

% To further enhance efficiency, the tool employs a pruning strategy based on a predefined action dependency graph (Supplementary Note~\ref{subsubsection:appendix-action-dependency-graph}), which eliminates invalid actions before the \textbf{\textit{Expansion}} phase.
% % The tool also incorporates a pruning strategy that leverages a predefined action dependency graph to reduce computational overhead by eliminating invalid actions before \textbf{\textit{Expansion}} (Supplementary Note~\ref{subsubsection:appendix-action-dependency-graph}).     

% \begin{figure}[H]
%     \centering
%     \includegraphics[width=1\linewidth]{figures/a-star.jpg}
%     \caption{
%         The framework of \toolname{action\_selection()} tool. 
%         It includes "three phases: (a) selection, (b) expansion, and (c) update. The dark and grey circles indicate the explored actions and the potential but unexplored ones, respectively. The blue circles represent the selected next step."
%         \wyf{TODO: re-draw this figure, and move this figure to SN.}
%     }
%     \label{fig:a-star}
% \end{figure}




% \subsection{Inter-Figure Coordination}
% \label{subsection:si-cross-figure-coordination}
% \wyf{[TODO: (1) add above statements based on final implementation: data-point level and aggregation-level filtering. (2) map to figure~\ref{fig:bidirectional-mapping}: workspace DB, coordination template, and update template when coordinating.]} 

% \newlyadded{To claim: our method both fit drill-down (case II and science policy) and bottom-up (case climate):
% (1) drill-down: filter workspace table by filtering criteria, and obtain individual data point IDs or filtered group IDs for further filtering; 
% (2) bottom-up: not limit to first filter the workspace table (can select other tables). But use the filtering criteria to filter data. 
% \textbf{One limitation: currently for the workspace table: we only upload the chart data tables -- which may not include scenarios for data analysis (Python code) scenarios (yifang: think it clearly again).}
% }

% \newlyadded{we specifically designed a function to classify the extended chart generation type, to control the selection of proper tables (workspace for drill-down vs. other raw tables for bottom-up). Input context: ego chart title and description, all tables (including eco-chart workspace table), check extended chart generation api}

% \newlyadded{Coordination: should include not only SQL template, but rather a list of action and its code, in order to deal with more complex scenarios (science policy case: topic summary).}

% \wyf{[Yifang TODO]: add a new row in Figure 1 two show this bi-directional mapping. Two types of scenarios: aggregated level data and individual-level id based data in workspace tables. Or, add a figure in method - action space.}


% \subsection{\newlyadded{Prompt Design}} 
% \label{subsection:si-prompt-design}
% We employ four prompt engineering techniques to optimize our multi-agent workflow performance~\cite{white2023prompt, sahoo2024systematic}: 

% \begin{itemize}
%     \item \textbf{(1) Structured XML formatting.} 
%     We develop a suite of XML tags to compartmentalize prompt components, such as \code{<roles>}, \code{<instructions>}, and \code{<constraints>} (Fig.~\ref{fig:prompt-design}), to increase the clarity, accuracy, and parseability~\cite{PromptXML, sahoo2024systematic}. 
%     % This structured approach improves LLM comprehension and response consistency across different agent interactions.
%     % (1) Tag definition for agents
%     % (2) Tag definition for tools
%     % (3) Shared tags 
%     % - Define roles. 
%     %     - https://docs.anthropic.com/en/docs/build-with-claude/prompt-engineering/system-prompts 
%     % - XML tags
%     %     - Todo: we should define and a table to include all tags used in agents and tools. 
%     %     % - https://docs.anthropic.com/en/docs/build-with-claude/prompt-engineering/use-xml-tags#why-use-xml-tags
%     % Structured prompt: Use XML tags like <thinking> and <answer> to separate reasoning from the final answer.
%     % % https://docs.anthropic.com/en/docs/build-with-claude/prompt-engineering/chain-of-thought#example-financial-analysis-with-thinking
%     % OpenAI: https://platform.openai.com/docs/guides/text?api-mode=chat 
%     % - "Some prompt engineering techniques will work with every model, like using message roles."
%     % - You could think about developer and user messages like a function and its arguments in a programming language.
%     %     - developer messages provide the system's rules and business logic, like a function definition.
%     %     - user messages provide inputs and configuration to which the developer message instructions are applied, like arguments to a function.
%     % Let Claude think (chain of thought prompting) to increase performance
%     %     % - https://docs.anthropic.com/en/docs/build-with-claude/prompt-engineering/chain-of-thought#example-writing-donor-emails-basic-cot
%     %     % - No need in tool definition. But required in Planner Agent
%     % OpenAI: https://platform.openai.com/docs/guides/text?api-mode=chat 
%     % % GPT-4.1 Prompting Guide (https://cookbook.openai.com/examples/gpt4-1_prompting_guide) > `5. General Advice`

    % \item \textbf{(2) Chain-of-thought reasoning.}
    % We specifically use the \code{<internal_reasoning>} tag to guide the model work out a plan with step by step instructions, enhancing reasoning robustness and analytical coherence~\cite{wei2022chain}. 

    % \item \textbf{(3) Few-shot learning.}
    % We maintain an example library that enables dynamic retrieval and insertion of contextually relevant examples into prompt templates using the \code{<example>} tag, providing targeted guidance for diverse analytical scenarios~\cite{brown2020language}.
    % This modular separation maintains prompt conciseness and facilitates system maintenance and expansion as conversational history grows, ensuring scalable performance without compromising prompt clarity. 
    % \wyf{TODO: add examples (cite code repo?) for each agent and tool.}
    % % "Further refinements are introduced by Li et al. [30], who demonstrate that incorporating one-shot and few-shot learning approaches substantially enhances the accuracy and robustness of visualization generation, particularly in complex or ambiguous cases." -- PVIS2026 (Siming's paper > related work 2.2, intelligent drill-down)
    % % This type of separation (of an example library) keeps the original prompt short and clean and make it easier to maintain and expand when the user chat history increases. 
    % % for agents and tools to retrieve and insert into the prompt template with the \code{<example>} tag~\cite{brown2020language}. 
    % % This type of separation (of an example library) keeps the original prompt short and clean and make it easier to maintain and expand when the user chat history increases. 

%     \item \textbf{(4) Dynamic prompting.}
%     Beyond static contents, we incorporate variable contents into the prompts, such as user input (both natural language and direct manipulation), conversational context (\eg, chat history, data context, and RAG-retrieved knowledge), and few-shot learning examples, which allows more precise user intent interpretation and contextually relevant responses~\cite{sahoo2024systematic}.  
%     % Future work: 
%     % - 每次对这个文件retrieve 3个最相关的example
%     % - Prefill Claude's response for greater output control 
%     %     - TODO
% \end{itemize}

% \begin{figure}[H]
%     \centering
%     \includegraphics[width=1\linewidth]{figures/prompt-design.png}
%     \caption{This is an example figure. \wyf{[Yifang TODO]: replace with our own structure.}}
%     \label{fig:prompt-design}
% \end{figure}



% \subsection{\newlyadded{Context Design}}
% \label{subsection:appendix-context-design}
% The iterative data exploration process and multi-modal outputs (\eg, data, code, and visualization) present challenges to deal with long context during the multi-agent workflow. 
% We design several stratifies to address this problem. 

% \begin{itemize}
%     % (1) Within one QA round
%     \item \textbf{(1) Single-round conversation management.}
%     We developed a structured data context format for individual question-answer cycles that stores only essential information about action sequences, including action indices, objectives, execution status, results, evaluation scores, rationale, and remaining tasks. 
%     \wyf{[Yifang TODO]: add a code snapshot; and how to optimize it (rather than store all the data, we store a small sample-double check).}
%     % current_data_context = (
%     %     "*********\n"
%     %     f"Step {action_index}: {action}\n"
%     %     f"Goal: {actions[action]}\n"
%     %     f"Execution Status: {action_result['status']}\n"
%     %     f"Execution Result: {action_result['result']}\n"
%     %     # f"Global Condition Status Dict: {global_condition_status_dict}\n"
%     %     f"Evaluation: {score}\n"
%     %     f"Reason: {reason}\n"
%     %     f"Remaining Plans: {remaining_plans}\n"
%     % )
%     % This selective retention reduces context overhead while preserving critical workflow information. 
%     % we specifically design a data context format to deal with one round of conversation (one QA round). 
%     % Only the action sequence will be stored during the process, including action index, goal, action execution status (whether success or failure), action results, evaluation score, reason, and remaining tasks and plans (Supplementary Note~\ref{subsection:appendix-data-context-design}). 

%     % (2) Semantic context
%     \item \textbf{(2) Cross-session semantic compression.}
%     \wyf{For conversations spanning multiple question-answer rounds or cross-sessions, we employ automated summarization to compress chat history into concise paragraph-form representations.} 
%     % This approach maintains contextual coherence while preventing context window overflow, enabling sustained analytical workflows without performance degradation. 
%     % For one chat session across different QA round and cross-session contexts, we summarize the chat history into a paragraph to compact the context. 
%     % Note: Specifically, in addition to traditional chat history, we've 
%     % 3-2 integrate vision language model (vis code and image) to infer insights and recommend next-step exploration. 
%     % 3-3 只展示重要的reasoning信息，to avoid overwelming 例如action_name, result (SQL code, python code, vega-lite code, dataframe, vis image, ...) 
%     % - Long context prompting tips
%     %     - TODO: may need to add chat history summary
%     %     - https://docs.anthropic.com/en/docs/build-with-claude/prompt-engineering/long-context-tips
% \end{itemize}

% \subsection{\newlyadded{Database Design}} 
% \label{subsection:si-db-design} 
% We have designed a user management database tailored to support LLM-native figures and data driven artifact. 
% The data tables and schema are shown in the figure below (Fig.~\ref{fig:user-chat-history-artifact-management}). 

% \wyf{TODO: add definition of all columns.}

% \begin{figure}
%     \centering
%     \includegraphics[width=1\linewidth]{figures/database-schema-artifact-management.png}
%     \caption{Database schema to store data-driven artifact, allowing for storing the chart extension and manipulation history in a more structured way. 
%     }
%     \label{fig:user-chat-history-artifact-management}
% \end{figure}



% \subsection{\newlyadded{Computational Evaluation}} 
% \label{subsection:si-computational-evaluation}

% Round-trip reproducibility. 
% % Note: 我们并没有重跑case
% % TODO: 给2个例子：1. 重新跑那个embedding结果，贴2个scatter plot：表示结果有些许不同;2. 重跑一个简单的case，画一个pipeline，表示所有数据都存储了，所以最后两个figure结果是一样的。


% % % \wyf{Note: we do not need to emphasize "update_chart" here, because we do not have any GUI selection here. Not our focus. But we can report results in SI and discuss limitations and future works: very complex, LLM fails in choosing the correct table at the very beginning (e.g., "Show the top 10 researchers by number of papers published": directly choose workspace table which only has 10 records)}

% We evaluate correctness of the generated code (SQL query, Python code, and Vega-Lite specification), the retrieved data subset $D$, and the resulting figures through manual inspection by two authors and cross-validated with the generated LLM-based solution.
% % \wyf{notice: for 1st question: for each question, remember to remove duplicate questions (only two criteria: exactly the same, and only differ in the first word.)}

% % Binglu: 实验的图就是很简单，一般想搞复杂就分类别画，做 heterogeneous analysis

% Additionally, for each question, we run the same user instruction and interaction for $3$ times to test the stability of our LLM framework.

% % multi-agent workflow stability: test the same question multiple times
% \wyf{We can directly use the 1st question generation (some repeat many times), 2nd question, to validate, no need to rerun the test. 
% Or, we can sample 10\% of the cases to re-run. -- to put into SI.}


% We validate the results manually with two authors. 
% Steps: 
% each author will validate all the cases in three parts:
% 1. first figure generation (including whether successfully generate a chart, and condition on this, whether correctly generate SQL, Python, and Vega-Lite)
% 2. second figure generation
% 3. coordination between figures.

% % 3. repeat 3 times
% To assess robustness under stochastic LLM behavior, we repeat each test case \textbf{three times} with identical inputs and report the consistency of mapping outcomes across runs. 

% \newlyadded{
% We use LLM to generate 398 test cases to evaluate our proposed demo system \systemname. 
% Then we manually examine the questions, chart types, and interactions of these cases, and remove duplicated cases that:
% 1. two question strings, chart types, interaction types: all are the exactly the same;
% 2. two question strings: allow the first word: show difference. But other words should be exactly the same. 
% % code: sciscicanvas/sciscicanvas-backend/data/case-study-2-InnovationInsights-NU-computational-evaluation-dataset-20251217/phase-3-test-all-set-400-questions-20250113/1-preprocess-400-questions-20250115.ipynb
% \wyf{Note: double check removed cases, add those with "similar" but not "exact the same" cases back to the test set.} 
% In addition, we also filter out those with no semantic meaning or interaction semantic meaning under SciSci context. 
% For example, the first chart requires brush the year range, while the second chart asks to collect data from all years -- the GUI interaction is then useless (1st question: "Display the temporal trend of number of papers with NIH grants by publication year (using a line_chart), 2nd question: "Compare the average NIH grant counts across all years with the selected year range (using a bar_chart)").
% \wyf{TODO: invite yifan and erzhuo to cross validate these questions.}
% } 
% \wyf{For questions with fuzzy answers, we still keep the question to see how LLM will automatically measure the problem with some metrics.}
% We also keep cases with similar semantic meaning but different expression, and regard them as different cases \wyf{(add justification; and also add a number/proportion of these cases)}.
% The total number of valid cases is 305.

% Note: in order to generate and test interactions for diverse chart types, we explicitly specify the chart type for chart generation (e.g., \textit{``'Show me the relationship between team size and science citations for all papers \wyf{(using a scatter plot)}''}).

% Note: some of the ticks of x axis in temporal charts does not show number of years (e.g., 2005) but rather 0.2 etc. This is because we did not explictly deal with it in \actionname{add_encoding} channel.
% % 现在x encoding是："type": "temporal"
% % 只要改成这样就行：
% % "x": {
% %   "field": "paper_year",
% %   "title": "Publication Year",
% %   "type": "quantitative",
% %   "axis": { "format": "d", "tickMinStep": 1 }
% % }

% Note: a set of questions in Q2, like case 169, 
% % "冗余of join ws, but ok;
% % Note: 没有保留Q1的filtering: with news_mentions
% % A better solution: let LLM to infer whether to keep previous question's context, or just keep the filtering criteria from the chart"

% \wyf{Note: we have added some cases for refining an existing chart. Problem: we have not define clearly what does "refine" a chart mean: (1) transform existing data attribute? (2) add new data attribute but does not change chart type? (3) add annotation? ...}


% Using datasets in the case study, we ask LLM to generate a list of test cases and each case is defined by a first initial question and a follow-up question pair. 
% For both questions, we ask LLM to generate as diverse cases as possible according to the following dimensions: 
% diverse figure types (\eg, bar charts, line charts, scatter plots, and pie charts), interaction types (\eg, single-mark clicks and 1D and 2D brushes), question difficulty levels/tiers (\ie, Tier-1 (canonical/simple) scenarios, involving a single raw data table with no or a few transformations; and Tier-2 (realistic/complex) scenarios, involving multiple tables and more sophisticated data transformations and analytical operations), and high-level solution logic to answer the question (as the reference for manual checking the results). 
% Please refer to the supplymentary information for example cases \wyf{(Sec.~\ref{subsection:si-computational-evaluation})}.
% \wyf{[Yifang]: to discuss whether to split into drill-down and bottom-up.}

% Each test case is defined by a <figure type, interaction type> pair.
% given the dataset and table description, we ask LLM to generate a list of questions for each type of (figure_type, interaction_type, tier_type)
% Using datasets in the case study, we generate a suite of visualizations for which ground-truth correspondences between visual marks and data rows are known. 
% These include: 
% bar charts,
% line charts,
% scatter plots, 
% and pie charts. 
% bar charts (single/grouped),
% line charts (single/multi-series),
% scatter plots with color encodings, 
% pie charts, 
% faceted visualizations. 
% For each chart, we programmatically generate a set of interactions, including single-mark clicks and 1D and 2D brushes. 
% combined selections across marks or facets. 






% \begin{table}[t]
% \centering
% \caption{
% \newlyadded{Performance summary of mapping fidelity accuracy: visualization -> analytical operation} 
% }
% \label{tab:example}
% \begin{tabularx}{\linewidth}{llXc}
% \toprule
% Chart Type & Interaction Type & Test Case & Result \\
% \midrule

% % 假设 Scatter Plot 总共 5 行（3 + 2）
% \multirow{5}{*}{Scatter Plot}
%   & \multirow{3}{*}{Single Click}
%   & Tier-1. Case Study (Fig.~\ref{fig:case-1}). Follow-up question:
%     \textit{``Give me a raw data table of this researcher''}. & Correct \\
%   & 
%   & Tier-2. Case Study (Fig.~\ref{fig:case-1}). Follow-up question:
%     \textit{\newlyadded{``For each publication year, what is the total number of patent citations received by this researcher’s papers?''}}. & Correct \\
    
%   & \multirow{2}{*}{2D Brush}
%   & Tier-1. Case Study (Fig.~\ref{fig:case-1}). Follow-up question:
%     \textit{``Show me the gender distribution''}. & Correct \\
%   & 
%   & Tier-1. Case Study (Fig.~\ref{fig:case-1}). Follow-up question:
%     \textit{``Show me the department distribution''}. & Correct \\
%   & 
%   & Tier-2. Case Study (Fig.xxx, Science Policy). Follow-up question:
%      \textit{{\newlyadded{``Summarize the topic of these papers.''}}}. & Correct \\
%   % & Tier-2. Case Study (Fig.~\ref{fig:case-1}). Follow-up question:
%   %   \textit{{\newlyadded{``What is the distribution of patent assignee types (such as company assignees or university assignees)''}}}. & Correct \\

% \multirow{1}{*}{Line Chart}
%   & \multirow{2}{*}{1D Brush}
%   & Tier-1. Climate Example (Fig.~\ref{fig:bidirectional-mapping}). Follow-up question: 
%   \textit{``Show me the average temperature of each U.S. state during the selected time range, and rank them from hottest to coolest''}. & Correct \\
%   &
%   & Tier-2. 
%   \textit{``xxxxxxx''}. & Correct \\

% \multirow{1}{*}{Bar Chart}
%   & \multirow{2}{*}{1D Brush}
%   & Tier-1. Case Study (Fig.~\ref{fig:case-1}). Follow-up question:
%     \textit{``xxxxxxx''}. & Correct \\
%   & 
%   & Tier-2. Case Study (Fig.~\ref{fig:case-1}). Follow-up question:
%     \textit{``xxxxxxx''}. & Correct \\
  
% \multirow{1}{*}{Pie Chart}
%   & \multirow{2}{*}{Single Click}
%   & Tier-1. Case Study (Fig.~\ref{fig:case-1}d). Follow-up question:
%     \textit{``xxxxxxx''}. & Correct \\
%   & 
%   & Tier-2. Case Study (Fig.~\ref{fig:case-1}). Follow-up question:
%     \textit{``xxxxxxx''}. & Correct \\ 

% \bottomrule
% \end{tabularx}
% \end{table}

% \begin{table}[t]
% \centering
% \caption{
% \newlyadded{Example of test cases of mapping fidelity accuracy: visualization -> analytical operation} 
% }
% \label{tab:example}
% \begin{tabularx}{\linewidth}{llXc}
% \toprule
% Chart Type & Interaction Type & Test Case (First Question) & Test Case (Follow-up Question) & Result \\
% \midrule

% % 假设 Scatter Plot 总共 5 行（3 + 2）
% \multirow{5}{*}{Scatter Plot}
%   & \multirow{3}{*}{Single Click}
%   & Tier-1. First question: \textit{``Show me the relationship between number of papers and number of patents for all researchers''}. & Tier-2. Follow-up question: \textit{``Apply log transformation to both axes to better visualize the distribution''}. & Correct \\
    
%   & \multirow{2}{*}{2D Brush}
%   & Tier-2. First question: \textit{``Show me the relationship between disruption score and science citations for papers published after 2010''}. & Follow-up question: \textit{``Show me the field distribution of the selected papers''}. & Correct \\
% \bottomrule
% \end{tabularx}
% \end{table}
